# Supplementary material for: On the use of higher order waveforms in the search for gravitational waves emitted by compact binary coalescences
Source: arXiv:1102.1749 source file (2011-10-17)
Supplement: Supplementary file 1 [file AppendixC.tex]

\chapter{How to search for gravitational waves from CBC}
\label{AppendixC}
\lhead{Appendix . \emph{How to search for gravitational waves from CBC}}
\rule{15.7cm}{0.05cm}
